# Supplementary material for: Mapping Phase Diagrams of Quantum Spin Systems through Semidefinite-Programming Relaxations
Source: arXiv:2507.03137 source file (2026-02-10)
Supplement: Supplementary file 1 [file suppmat.pdf]

# Supplementary Material for "Mapping phase diagrams of quantum spin systems through semidefinite-programming relaxations"

David Jansen, Donato Farina, Luke Mortimer, Timothy Heightman, Andreas Leitherer, Pere Mujal, Jie Wang, and Antonio Acín

## DETAILS ON THE SEMIDEFINITE PROGRAM

In all calculations, we exploit translation invariance in the $x$ direction for the one-dimensional chain (see Ref. [S1]) and in the $x$ and $y$ directions for the two-dimensional bilayer systems. We also exploit that Pauli strings can be reduced to their normal form (NF) as in Ref. [S1]. For example, for a one dimensional chain, $\mathrm{NF}(\hat{u}) = c\hat{\sigma}_{i_1}^{\alpha_1}\hat{\sigma}_{i_2}^{\alpha_2}\ldots\hat{\sigma}_{i_n}^{\alpha_n}$ with $c \in \{1, -1, \mathbf{i}, -\mathbf{i}\}$ and $1 \leq i_1 < i_2 < \ldots i_n \leq L$ for a Pauli string $\hat{u}$ and $\mathbf{i}$ being the imaginary unit. For formulating the SDPs with complex numbers, we follow Ref. [S2]. The calculations were done on an 11th-generation Intel(R) Core(TM) i5-11500 @ 2.70GHz processor with 128G RAM and an Intel(R) Xeon(R) Gold 6348 CPU @ 2.60GHz with 755G RAM.

### Positivity of reduced density matrices

In all simulations, we enforce that several $n$-site reduced density matrices are positive semidefinite:

$$\hat{\rho}_{i_1,\ldots,i_n} = \frac{1}{2^n}\left(\sum_{\alpha_1,\ldots,\alpha_n} \langle \hat{\sigma}_{i_1}^{\alpha_1}\ldots\hat{\sigma}_{i_n}^{\alpha_n}\rangle \, \hat{\sigma}_{i_1}^{\alpha_1}\ldots\hat{\sigma}_{i_n}^{\alpha_n}\right) \succcurlyeq 0\,, \tag{S.1}$$

with $\hat{\sigma}_{i_j}^{\alpha_j} \in \{\mathbb{1}, \hat{\sigma}_x, \hat{\sigma}_y, \hat{\sigma}_z\}$. This has been shown to significantly improve the bounds [S1, S3].

### Symmetries, monomials, and reduced density matrices for the transverse field Ising model

We choose the set of monomials $\mathcal{B}_d$, such that for $d \geq 1$, we include $\hat{\sigma}_i^\alpha$ for $i \in \{1,\ldots,L\}$ and $\alpha \in \{x,y,z\}$, for $d \geq 2$ we further include $\hat{\sigma}_i^\alpha\hat{\sigma}_{i+j}^\beta$ for $i \in \{1,\ldots,L\}$, $j \in \{1,\ldots,r\}$, and $\alpha,\beta \in \{x,y,z\}$, and for $d \geq 3$, we further include $\hat{\sigma}_i^\alpha\hat{\sigma}_{i+1}^\beta\hat{\sigma}_{i+2}^\gamma$ for $i \in \{1,\ldots,L\}$, and $\alpha,\beta,\gamma \in \{x,y,z\}$. For the data shown in the main text, we choose $d = 3$. Additionally, we exploit that the Hamiltonian $\hat{H}$, is invariant under

$$(\hat{\sigma}_i^x, \hat{\sigma}_i^y, \hat{\sigma}_i^z) \to (\hat{\sigma}_i^x, -\hat{\sigma}_i^y, \hat{\sigma}_i^z), \quad \forall i \in \{1,\ldots,L\}\,, \tag{S.2}$$

so that $\langle\hat{o}\rangle = 0$ if $\langle\mathrm{NF}(\hat{o})\rangle$ is variant under (S.2) [S1]. Note that we intentionally do not resolve symmetries that would enforce $\langle\hat{\sigma}_i^z\rangle = 0$ in order to detect the spontaneous symmetry breaking. We further enforce that the following reduced density matrices $\hat{\rho}_{i_1,\ldots,i_n}$ are positive semidefinite: $(i_1,\ldots,i_n) \in \{(1,j)$ for $j \in \{2,\ldots,L/2\}$, $(1,2,3)$, $(1,2,3,4)$, $(1,2,3,4,5)$, $(1,2,3,4,5,6)\}$.

### Symmetries, monomials, and reduced density matrices for the bilayer models

For the bilayer systems, we follow Ref. [S1] and utilize the sign symmetry of the model, the sign symmetry of the Hamiltonian, and the permutation symmetry. Furthermore, we exploit the $D_8$ symmetry in each layer and that the system is invariant under exchanging the two layers.

We choose the set of monomials $\mathcal{B}_d$ as follows: We always include $\hat{\sigma}_{a,i,j}^\alpha$ with $a \in \{1,2\}$, $i,j \in \{1,\ldots,L\}$, and $\alpha \in \{x,y,z\}$. For $d \geq 2$, we also include $\hat{\sigma}_{a,i,j}^\alpha\hat{\sigma}_{b,i+r_1,j+r_2}^\beta$ with $a,b \in \{1,2\}$, $i,j \in \{1,\ldots,L\}$, $r_1, r_2 \in \{-r,\ldots,r\}$, and $\alpha,\beta \in \{x,y,z\}$. For $d \geq 3$, we also include $\hat{\sigma}_{1,i,j}^\alpha\hat{\sigma}_{1,i,j+1}^\beta\hat{\sigma}_{1,i,j+2}^\gamma$, $\hat{\sigma}_{1,i,j}^\alpha\hat{\sigma}_{1,i,j+1}^\beta\hat{\sigma}_{2,i+1,j+1}^\gamma$, $\hat{\sigma}_{2,i,j}^\alpha\hat{\sigma}_{1,i+1,j}^\beta\hat{\sigma}_{2,i+2,j+1}^\gamma$, with $\alpha,\beta,\gamma \in \{x,y,z\}$ and $i,j \in \{1,\ldots,L\}$. For $d \geq 4$ we also include $\hat{\sigma}_{1,i,j}^\alpha\hat{\sigma}_{2,i,j}^\beta\hat{\sigma}_{1,i+1,j+1}^\gamma\hat{\sigma}_{2,i+1,j+1}^\eta$ with $i,j \in \{1,\ldots,L\}$ and $\alpha,\beta,\gamma,\eta \in \{x,y,z\}$.

Furthermore, we enforce that the reduced density matrices on the following sites are positive semidefinite $(i_1,\ldots,i_n) : ([a,i,j],[b,l,m])$ with $i,j,l,m \in \{1,\ldots,L\}$ and $a,b \in \{1,2\}$ for $o_{\mathrm{rdm}} \geq 2$, for $o_{\mathrm{rdm}} \geq 3$, we also include

$$\begin{aligned}
&([1,1,1],[1,2,1],[1,2,2]),\\
&([1,1,1],[2,1,1],[1,2,1]),\\
&([1,1,1],[2,2,2],[1,2,1]),\\
&([1,1,1],[2,1,2],[2,3,1]),
\end{aligned}$$

and for $o_{\mathrm{rdm}} \geq 4$, we also include

$$\begin{aligned}
&([1,1,1],[1,2,1],[1,3,1],[1,3,1]),\\
&([1,1,1],[2,1,1],[1,2,2],[2,2,2]),\\
&([1,1,1],[1,2,2],[1,3,1],[2,4,2]),
\end{aligned}$$

for $o_{\mathrm{rdm}} \geq 5$, we also include

$$\begin{aligned}
&([1,1,1],[2,1,1],[1,2,2],[2,2,2],[1,3,3]),\\
&([1,1,1],[2,1,1],[1,2,2],[2,2,2],[2,3,3]),\\
&([1,1,1],[2,1,1],[1,2,2],[2,2,2],[2,4,3]),
\end{aligned}$$

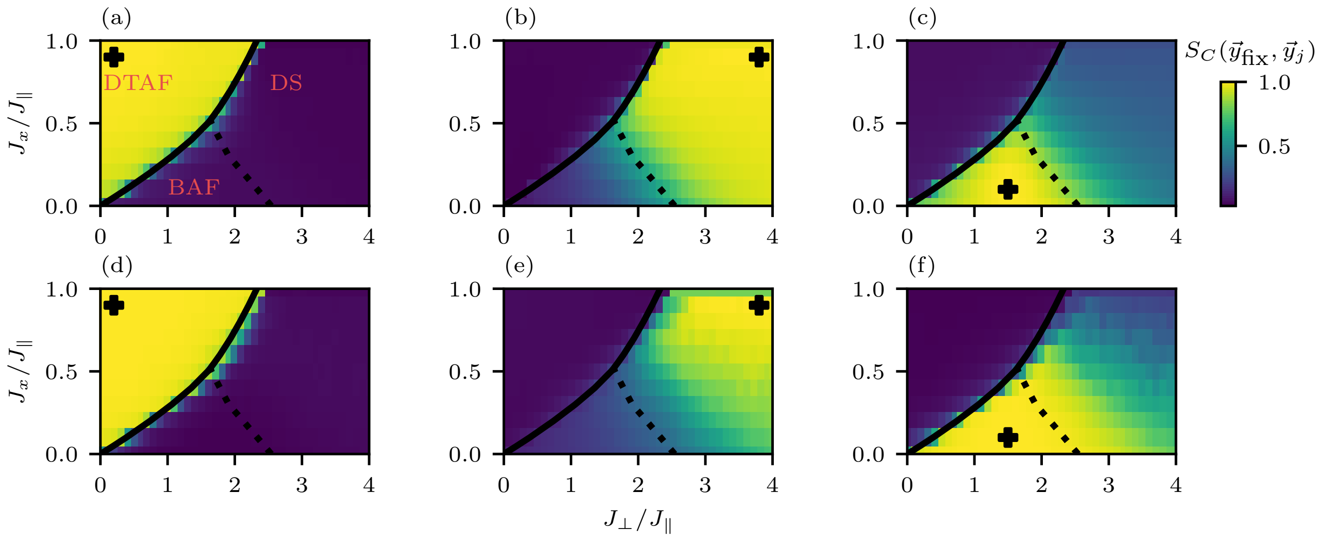


Figure S1. Phase diagrams of the FBH model using the cosine similarity for different set of monomials $\mathcal{B}_d$ for $L = 6$. (a)-(c) $d = 4$, $r = 3$, and $o_{\text{rdm}} = 6$. (d)-(f) $d = 2$, $r = 2$, and $o_{\text{rdm}} = 2$. The black crosses indicates the values chosen for $\vec{y}_{\text{fix}}$.

and for $o_{\text{rdm}} \geq 6$, we also include

$$([1,1,1],[1,2,1],[1,3,1],[1,4,1],[1,5,1],[1,6,1]),$$
$$([1,1,1],[1,1,2],[2,2,2],[1,3,3],[1,3,4],[1,4,4]),$$
$$([2,1,1],[1,2,1],[2,3,2],[2,2,2],[1,3,2],[2,4,3]).$$

How the selection of the monomials and reduced density matrices influences the phase diagram can be seen in Fig. S1. There, we observe that the phase boundaries are much closer to those in Ref. [S4] when $d = 4$, $r = 3$, and $o_{\text{rdm}} = 6$.

[S1] J. Wang, J. Surace, I. Frérot, B. Legat, M.-O. Renou, V. Magron, and A. Acín, Certifying ground-state properties of many-body systems, Phys. Rev. X **14**, 031006 (2024).

[S2] J. Wang, A more efficient reformulation of complex SDP as real SDP, arXiv:2307.11599 (2023).

[S3] L. Mortimer, D. Farina, G. Di Bello, D. Jansen, A. Leitherer, P. Mujal, and A. Acín, Certifying steady-state properties of open quantum systems, arXiv:2410.13646 (2024).

[S4] J. Stapmanns, P. Corboz, F. Mila, A. Honecker, B. Normand, and S. Wessel, Thermal critical points and quantum critical end point in the frustrated bilayer heisenberg antiferromagnet, Phys. Rev. Lett. **121**, 127201 (2018).
